# Supplementary material for: A Framework for Joint Design of Pilot Sequence and Linear Precoder
Source: arXiv:1210.1470 source file (2012-10-04)
Supplement: Supplementary file 1 [file appendix.tex]

%\subsection{Proof of Lemma~\ref{lem:envelope}}   \label{proof:lem:envelope}
%
%The Pareto boundary $\partial^+\Bs(\mathcal{P},\mathcal{Q})$ is the envelope of the family of simplices $\Bs(\BP,\mathcal{Q})$ parametrized by $\BP$, or---to be more precise---of the family of planes $\partial^+\Bs(\Bp,\partial\mathcal{Q})$ delimiting said simplices. From \eqref{simplex_vertices} it can be shown that these planes are parametrized as $\sum_i \frac{s_i}{\omega_i} = 1$, where $\omega_i = [\Bomega]_i$ are the non-decreasingly ordered values [cf.~\eqref{generalized_evp}]
%\begin{align}
%	\omega_{\pi_\omega(i)} = \frac{\hat{r}_i(p_i)}{\mu_\mathcal{Q}^{-1} + \tilde{r}_i(p_i)}
%\end{align}
%where $\pi_\omega$ is an appropriate ordering permutation. By inserting the latter expression into $\sum_i \frac{s_i}{\omega_i} = 1$, the family of planes may be represented by an equation $F_\Bp(\Bs) = 0$ with
%\begin{align}   \label{family_of_lines}
%	F_\Bp(\Bs)
%	&= \sum_i \frac{s_i}{\omega_i} - 1 \nonumber\\
%	&= \biggl( \sum_i s_i \frac{\mu_\mathcal{Q}^{-1} + \tilde{r}_i(p_i)}{\hat{r}_i(p_i)} \biggr) - 1.
%\end{align}
%The envelope of this family of curves is given by the $\Bs$'s fulfilling the envelope equation
%\begin{align}   \label{envelope_equation}
%	F_\Bp(\Bs) = \frac{\partial}{\partial \epsilon} F_{\Bp + \epsilon\Bdelta}(\Bs) = 0
%\end{align}
%for any $\Bp \geq \mynull$ and $\Bdelta$ such that $\myone^\Tr\Bp = \mu_\mathcal{P}$ and $\myone^\Tr\Bdelta = 0$.
%
%The pilot and precoder allocations shall be represented respectively as $\Bp = [p_1,\mu_\mathcal{P}-p_1]^\Tr$ and $\Bq = [q_1,\mu_\mathcal{Q}-q_1]^\Tr$ with the parameter pair $(p_1,q_1) \in [0;\mu_\mathcal{P}] \times [0;\mu_\mathcal{Q}]$. The function $F_\Bp$ is parametrized by a single scalar $p_1$, so we write $F_{p_1}$ instead:
%\begin{align}   \label{envelope_equation_first}
%	F_{p_1}(\Bs)
%	&= s_1 \frac{1+r_1(p_1 + \mu_\mathcal{Q})}{r_1^2 \mu_\mathcal{Q} p_1} \nonumber\\
%	&\qquad { } + s_2 \frac{1+r_2(\mu_\mathcal{Q}+\mu_\mathcal{P}-p_1)}{r_2^2 \mu_\mathcal{Q} (\mu_\mathcal{P}-p_1)} - 1.
%\end{align}
%The partial derivative $\frac{\partial}{\partial p_1}F_{p_1}$ reads as
%\begin{align}   \label{envelope_equation_second}
%	\frac{\partial F_{p_1}}{\partial p_1}
%	= s_2 \frac{1+r_2\mu_\mathcal{Q}}{r_2^2\mu_\mathcal{Q}} \frac{1}{(\mu_\mathcal{P}-p_1)^2} - s_1 \frac{1+r_1\mu_\mathcal{Q}}{r_1^2\mu_\mathcal{Q}} \frac{1}{p_1^2}.
%\end{align}
%Assuming that we want to find the envelope point $(s_1,s_2)$ for a given $p_1$, the envelope equation \eqref{envelope_equation} boils down to a system of two equations in $\Bs$, namely
%\begin{align}   \label{envelope_equation_as_system}
%	\begin{bmatrix}
%		F_{p_1}(\Bs) \\
%		\frac{\partial}{\partial p_1} F_{p_1}(\Bs)
%	\end{bmatrix}
%	= \mynull.
%\end{align}
%With Expressions~\eqref{envelope_equation_first} and \eqref{envelope_equation_second}, this is nothing else than a linear equation of the form $\BA\Bs = \Be_1$, where the matrix $\BA = \left[ \begin{smallmatrix} a_{11} & a_{12} \\ a_{21} & a_{22} \end{smallmatrix} \right]$ is
%\begin{align}
%	\BA =
%	\begin{bmatrix}
%		\frac{1+r_1(p_1 + \mu_\mathcal{Q})}{r_1^2 \mu_\mathcal{Q} p_1} &
%		\frac{1+r_2(\mu_\mathcal{Q}+\mu_\mathcal{P}-p_1)}{r_2^2 \mu_\mathcal{Q} (\mu_\mathcal{P}-p_1)} \\
%		-\frac{1+r_1\mu_\mathcal{Q}}{r_1^2\mu_\mathcal{Q}} \frac{1}{p_1^2} &
%		\frac{1+r_2\mu_\mathcal{Q}}{r_2^2\mu_\mathcal{Q}} \frac{1}{(\mu_\mathcal{P}-p_1)^2}
%	\end{bmatrix}.  \end{align}
%As one can easily see, the entries $a_{11}$, $a_{12}$ and $a_{22}$ are positive, whereas $a_{21}$ is negative. Therefore, $\det(\BA) > 0$ and $\BA$ is non-singular on the open interval $p_1 \in (0;\mu_\mathcal{P})$. The envelope points are given by $\Bs = \frac{1}{|\BA|} [a_{22}, -a_{21}]^\Tr$. By reverting Equation~\eqref{s_vectorial},
%\begin{align}   \label{q_vectorial}
%%	q_i = \frac{s_{\pi_s(i)} \hat{r}_i^{-1}}{1 - \langle \tilde{\Br} , \BPi_s\Bs \odot \hat{\Br}^{-1} \rangle},
%	q_1 = \frac{s_1 \hat{r}_1^{-1}}{1 - \tilde{\Br}^\Tr (\Bs \odot \hat{\Br}^{-1})},
%\end{align}
%where `$\odot$' is the entrywise product. From writing out \eqref{q_vectorial} with $\Bs$ being given as the solution to the linear system \eqref{envelope_equation_as_system}, we end up with $q_1$ being a function of $p_1$:
%\begin{align}   \label{app:q1p1}
%%	\textstyle \beta
%%%	= \frac{\alpha(\frac{1}{Q} \!+\! r_2)(1 \!+\! r_1 \mu_\mathcal{P} \alpha)}{\alpha(\frac{1}{Q} \!+\! r_2)(1 \!+\! r_1 \mu_\mathcal{P} \alpha) \!+\! (1 \!-\! \alpha)(\frac{1}{Q} \!+\! r_1)(1 \!+\! r_2 \mu_\mathcal{P} (1 \!-\! \alpha))}.
%%	= \textstyle \frac{\alpha(1 + r_2 \mu_\mathcal{Q})(1 + r_1 \mu_\mathcal{P} \alpha)}{\alpha(1 + r_2 \mu_\mathcal{Q})(1 + r_1 \mu_\mathcal{P} \alpha) + (1 - \alpha)(1 + r_1 \mu_\mathcal{Q})(1 + r_2 \mu_\mathcal{P} (1 - \alpha))}.
%	q_1(p_1)
%	= \textstyle \frac{\mu_\mathcal{Q} p_1(1 + r_2 \mu_\mathcal{Q})(1 + r_1 p_1)}{p_1(1 + r_2 \mu_\mathcal{Q})(1 + r_1 p_1) + (\mu_\mathcal{P} - p_1)(1 + r_1 \mu_\mathcal{Q})(1 + r_2 (\mu_\mathcal{P} - p_1))}.
%\end{align}
%The explicit parametrization~\eqref{explicit_border_parametrization} is obtained when writing out the expressions of the $s_i$ for two transmit antennas [cf.~\eqref{s_vectorial}] in full as
%\begin{subequations}
%\begin{align}
%	s_1 &= \frac{r_1^2 p_1 q_1 (1\!+\!r_2 p_2)}{(1\!+\!r_1 p_1)(1\!+\!r_2 p_2)\!+\!r_1 q_1 (1\!+\!r_2 p_2)\!+\!r_2 q_2 (1\!+\!r_1 p_1)} \\
%	s_2 &= \frac{r_2^2 p_2 q_2 (1\!+\!r_1 p_1)}{(1\!+\!r_1 p_1)(1\!+\!r_2 p_2)\!+\!r_1 q_1 (1\!+\!r_2 p_2)\!+\!r_2 q_2 (1\!+\!r_1 p_1)},
%\end{align}
%\end{subequations}
%and then inserting \eqref{app:q1p1} thereinto.
%
